# Supplementary material for: Trusted Container Extensions for Container-based Confidential Computing
Source: arXiv:2205.05747 source file (2022-05-11)
Supplement: Supplementary file 1 [file appendix.tex]

%!TEX root = ../main.tex

\section{Appendix}
\label{appendix}
\begin{lstlisting}[frame=single,caption={Example Secure Channel API Usage: Client},breaklines=true,captionpos=b,label={scclient},language=Golang,style=mystyle]
func main() {
	err := sclib.Register("TEST_CLIENT")
	if err != nil {
		log.Fatalln(err)
	}

	sclib.GetRegisteredVMs()

	owner, err := sclib.GetSelfOwner()
	if err != nil {
		log.Fatalln("Could not get my Owner certificate")
	}

	validOwners := []*x509.Certificate{owner}
	conn, err := sclib.Dial("TEST_SERVER", validOwners)
	if err != nil {
		log.Fatalln(err)
	}

	conn.Write([]byte("Hello from client"))
	buf := make([]byte, 32)
	n, err := conn.Read(buf)
	if err != nil {
		log.Fatalln(err)
	}
	buf = buf[:n]
	log.Println("Got from server: " + string(buf))

	conn.Close()
}
\end{lstlisting}

\begin{lstlisting}[frame=single,caption={Example Secure Channel API Usage: Server},breaklines=true,captionpos=b,label={scserver},language=Golang,style=mystyle]
func main() {
	sclib.Register("TEST_SERVER")
	sclib.GetRegisteredVMs()

	l, err := sclib.Listen()
	if err != nil {
		log.Fatalln(err)
	}
	
	for {
		conn, err := l.Accept()
		if err != nil {
			continue
		}

		buf := make([]byte, 32)
		n, err := conn.Read(buf)
		if err != nil {
			log.Fatalln(err)
		}
		buf = buf[:n]
		log.Println("Got from client: " + string(buf))

		conn.Write([]byte("Hello from server"))

		conn.Close()
	}
}
\end{lstlisting}
